# Supplementary material for: Global warming: Temperature estimation in annealers
Source: arXiv:1606.00919 ancillary file (2017-08-25)
Supplement: Supplementary file 1 [file TemperaturePaper_SupplementaryMaterial.pdf]

# *Supplementary Material*: Global warming: Temperature estimation in annealers

**Jack Raymond**[1,*], **Sheir Yarkoni**[1], **and Evgeny Andriyash**[1]
*Correspondence:
Jack Raymond
jraymond@dwavesys.com

## 1 OUTLINE

- In Section 2 we describe in detail common problem classes associated with D-Wave processors, but not presented in the main paper. These problem classes motivate some additional results throughout this text.
- Section 3 is devoted to the investigation of multi-canonical methods of temperature estimation. We implement and extend known methods, analyze results with respect to the DW2X, and finally show limitations of such methods.
- In Section 4 we explain thoroughly what one could expect from the DW2X as a sampler, and show how temperature is affected by embedding and spin-reversal transforms.
- Section 5 discusses a standard intepretation for the maximum log-pseudo-likelihood method.
- Section 6 shows how the self-consistent approximation method can be improved with increasingly powerful kernels.
- Section 7 explores a tractable method of evaluating KL-divergence.
- Section 8 presents AC3 results to complement the RAN1 results of Section M4.5.

For clarity, all figures and equations from the main text will be referenced throughout this text with the prefix “M”, e.g., “Figure M1”, “Eq. (M1)”, etc. Sections from this text will be regularly numbered, although figures and equations are referenced with the prefix “S”, as in “Figure S1”.

## 2 MODELS

In this paper we investigate multiple families of Ising spin problems of the form Eq. (M1). A number of exotic problem classes have been studied in the context of the DW2X [Hen et al. (2015); King et al. (2015a, 2016); Zhu et al. (2016)]. Many of the motivations for these classes relate directly to optimization, and involve manipulation of the *very* low energy landscape. We note that many of these manipulations do not lead to particularly interesting variations in the finite temperature properties (of which we are more concerned), except perhaps for small system sizes. As an example it is understood that all Chimera structured models with independent and identically distributed couplings will show the same finite temperature behavior, and no finite temperature spin glass transition, owing to universality [Katzgraber et al. (2014)]. Our model choices are chosen with the aim of demonstrating strong and varied ergodicity breaking effects at the scales studied. In the main text we have described RAN1 and AC3. Here we describe two additional models. Unpublished classes have also been studied, showing comparable phenomena.

## 2.1 Random Not-all-equal-3SAT

Random Not-All-Equal-3SAT (NAE3SAT) are a particular family of satisfiability problems closely related to 3SAT, and share the same computationally challenging features [Mezard and Montanari (2009); Douglass et al. (2015)]. We consider problems with $N$ variables and $M = 1.8N$ clauses. Each clause $m$ is described by 3 literals: a triplet of indices $\eta_{m,1}, \eta_{m,2}, \eta_{m,3}$ and a triplet of signs $a_{m,1}, a_{m,2}, a_{m,3}$ (a sign -1/+1 indicates a negative/positive literal). In random NAE3SAT, literals are selected independently: sampling uniformly the indices on $\{1, \ldots, N\}$, and the signs on $\pm 1$. In the models we generate we apply the further restrictions that (a) all problems we consider are satisfiable, (b) every variable appears in some clause and (c) all variables are dependent (the graph is connected). The configuration model can be used for sampling these topologies [Janson et al. (2000)].

An Ising model in which the ground states of energy $0$ are coincident with the satisfying assignments of NAE3SAT (true/false maps to +1/-1 ), and other states are assigned an energy equal to the number of clause violations, is described by the Hamiltonian

$$H(x) = \frac{1}{4} \sum_{m=1}^{M} \left[ a_{m,1} a_{m,2} x_{\eta_{m,1}} x_{\eta_{m,2}} + a_{m,1} a_{m,3} x_{\eta_{m,1}} x_{\eta_{m,3}} + a_{m,2} a_{m,3} x_{\eta_{m,2}} x_{\eta_{m,3}} - 1 \right] \tag{S1}$$

By expansion, we find the form in Eq. (M1) up to an unimportant constant offset. Finding ground states of this Hamiltonian solves an NP-complete satisfiability problem. However, the solution space structure at non-zero (but low) energies is also interesting in its own right when $M \gtrsim 1.5N$, paradigmatic of hard to sample from energy landscapes [Mezard and Montanari (2009)]. This hardness is due to the existence of a finite temperature random first order phase transition [Mezard and Montanari (2009); Landau and Binder (2005)].

The process of embedding can be used to generate an auxiliary problem that preserves the ground state properties, but is solvable by the DW2X [Cai et al. (2014)]. Data is only presented for the $40$ variable instances of the NAE3SAT problem, and for the DW2X parameterized to minimize TTS (see Section M4.4). The number of qubits required to represent the embedding problems fluctuates, and is determined automatically by the embedding procedure, but typically fits comfortably on an $8x8$ cell subgrid (C8) of the Chimera graph. Inference on the unembedded problem is possible by dynamic programming, whereas inference in the embedded problem requires parallel tempering MCMC.

Embedding, and transforming the samples obtained back into the logical space, can have important consequences for temperature estimation, as discussed in Section 4.5. The NAE3SAT problem is also used to demonstrate variation amongst locally-consistent estimators in Section 6.

## 2.2 The bidirectional associative memory (BAM) model

The bidirectional associative memory model is a neural network model without hidden units. It is the bipartite generalization of the Hopfield model [Bart (1988)]. In the model studied here, a set of $N$ Ising spins are divided into two equal groups that are conditionally independent, and a set of $M$ memories $\{\epsilon^{(m)}\}$ are drawn each independently and uniformly from $\{-1, +1\}^N$. If the model is trained to recall these memories under Hebbian learning, the learning procedure converges upon a distribution described by the Hamiltonian

$$H(x) = -\frac{2}{N} \sum_{i_1=1}^{N/2} \sum_{i_2=N/2+1}^{N} x_{i_1} x_{i_2} \sum_{m=1}^{M} \epsilon_{i_1}^{(m)} \epsilon_{i_2}^{(m)}. \tag{S2}$$

The BAM model has an easy to understand energy landscape when the number of memories to be stored is small compared to the number of variables $N$ [Tanaka et al. (2000)]. For large enough $N$ and $\beta > 1$ the Boltzmann distribution is defined by $2M$ well defined *modes* (these modes come in pairs related by a trivial symmetry). The memories $\pm\epsilon^{(m)}$ define the centers of these modes, and are local ground states (up to perhaps a small Hamming distance). This is a nice model for theoretical exploration since there is a clear distinction between the global features (modes), and local features. To be solved on DW2X (for more than 8 variables) the model would need to be embedded, but in this paper we only apply the STA to this model. A $128$ variable, $M = 3$ memory, model is studied in Section 3.4 to demonstrate interesting features of a multi-canonical approximation described in Section 3.

We apply the STA to the BAM model, choosing $\beta_T = 4$ and $200$ as the number of sweeps. The inverse temperature is chosen so as to be well above the known thermodynamic phase transition [Tanaka et al. (2000)], so that samples are well separated into modes. The number of sweeps is taken as $200$ so that in the STA distribution we observe large frequencies over many of the lowest energy states, in order that a simplified form of the Benedetti et al. method can be applied without distorting results qualitatively [Benedetti et al. (2016)].

## 3 MULTI-CANONICAL METHODS OF TEMPERATURE ESTIMATION

### 3.1 Multi-canonical maximum likelihood

Benedetti et al. recently described and applied a method of temperature estimation that exploited samples drawn from two or more annealer distributions, with application to the DW2X, where the distributions differed in a rescaling parameter [Benedetti et al. (2016)]. Methods such as this one are called *multi-canonical* since they involve samples drawn from multiple annealing distributions. In the main text we have focused on estimators that work on the basis of a single parameterization.

Suppose we are able to draw samples from an annealer at two different parameterizations ($A_1$ and $A_2$), each with distributions described by $P_{A_1}(x)$ and $P_{A_2}(x)$. The product distribution can be defined as $P_{A_1,A_2}(x_1, x_2) = P_{A_1}(x)P_{A_2}(x)$. If both are approximately Boltzmann, this product distribution will be close to $B_{\beta_1,\beta_2}(x_1, x_2) = B_{\beta_1}(x_1)B_{\beta_2}(x_2)$ for some pair $\beta_1$ and $\beta_2$. Estimating $\beta_1$ and $\beta_2$ by maximum likelihood reduces to two independent energy matching criteria (see Section M2.1). At this stage we have only doubled the work relative to the maximum likelihood estimator. However, suppose we make the assumption that $\beta_2$ is some known function of $A_1$ and $A_2$ given $\beta_1$. With this assumption we have sufficient information to determine both $\beta_1$ and $\beta_2$ from one energy matching criteria. Subtracting the conditions for $\beta_1$ from $\beta_2$ we obtain an energy gap matching criterion $\mathrm{EGM}(\beta_1, \beta_2) = 0$, with

$$\mathrm{EGM}(\beta_1, \beta_2) = \sum_{x_1,x_2} P_{A_1,A_2}(x_1, x_2)[H(x_1) - H(x_2)] - \sum_{x_1,x_2} B_{\beta_1,\beta_2}(x_2, x_1)[H(x_1) - H(x_2)] \; . \quad \text{(S3)}$$

The pair of equations $\mathrm{EGM}(\beta_1, \beta_2) = 0$ and $\beta_2 = f(A_1, A_2, \beta_1)$ defines our multi-canonical estimator.

One parameter that can be varied in the DW2X is a rescaling parameter $r$, which is comparable to the STA terminal temperature $\beta_T$ as discussed in Section M4.3[1]. Benedetti et al. [Benedetti et al. (2016)] proposed in their method to use two different values $r$, and assume that $\beta \propto r$, which in the context of annealers may hold for certain problems but not in general as shown in Section M4.5. The criterion we propose for

[1] In practice our DW2X rescaling parameter $r$ is a rescaling of the Hamiltonian submitted to the DW2X.

the multi-canonical method (S3) is not used in the approach of [Benedetti et al. (2016)], although both methods require an assumption on the response of $\beta$ to an annealing parameter.

The multi-canonical estimator has two drawbacks relative to the estimators previously discussed: we require two distributions from the annealer at different annealing parameters and we require an assumption about the response of the annealer temperature to changes in the annealing parameters. In Section 3.2 we explain how to apply the self-consistent approximation principle of section M3.1 to solve the energy gap matching criteria efficiently. In Section 3.3 we discuss the merits of multi-canonical methods. In section 3.2 we undertake a study analogous to that of Section M4.5, using our energy gap matching criteria. In Section 3.4 we implement a version of the Benedetti at al. method, and demonstrate how additional information can be teased out regarding local and global temperatures.

### 3.2 Multi-canonical statistics by self-consistency

In the case of the multi-canonical estimator of Section 3.1 we again must infer a mean energy difference between two Boltzmann distributions to evaluate the energy gap matching criterion, which is NP-hard. A kernel can again come to our rescue. This time we are inspired by the kernels from multi-canonical MCMC, such as parallel tempering [Hukushima and Nemoto (1996); Landau and Binder (2005)]; other choices that depend on the terminal temperatures (as opposed to simply the gap in the terminal temperatures) could also be considered. In effect we employ the following identity for Boltzmann samplers:

$$B_{\beta_1,\beta_2}(x_1, x_2) \propto B_{\beta_1,\beta_2}(x_2, x_1) \exp((\beta_1 - \beta_2)[H(x_1) - H(x_2)]). \tag{S4}$$

We complete the approximation by replacing $B_{\beta_1,\beta_2}(x_2, x_1)$ on the left of (S4) with a plug-in estimate $\hat{P}_{A_1,A_2}$ (M6) and substituting $B_{\beta_1,\beta_2}(x_1, x_2)$ into (S3)

$$\begin{aligned} \mathrm{EGM}(\beta_1, \beta_2) = \sum_{x_1,x_2} P_{A_1,A_2}(x_1, x_2)[H(x_1) - H(x_2)] - \\ \frac{\sum_{x_1,x_2} P_{A_1,A_2}(x_2, x_1) \exp\left\{(\beta_1 - \beta_2)[H(x_1) - H(x_2)]\right\} [H(x_1) - H(x_2)]}{\sum_{x_1,x_2} P_{A_1,A_2}(x_2, x_1) \exp((\beta_1 - \beta_2)[H(x_1) - H(x_2)])}. \end{aligned} \tag{S5}$$

The energy matching criterion can now be solved for $\Delta\beta = \beta_1 - \beta_2$, and will have a finite solution provided the energy distributions of the two annealing parameterizations overlap significantly. We expect an intermediate amount of overlap in the distributions is ideal to extract the maximum signal just as it is ideal for implementation of multi-canonical MCMC methods [Hukushima and Nemoto (1996); Landau and Binder (2005)]. Various works have considered how to extract maximal information from multi-canonical distributions, this could also inform a better choice of kernel [Shirts and Chodera (2008); Benedetti et al. (2016)].

If we know $\beta_1$ for annealer condition $A_1$ (or $\beta_2$ for annealer condition $A_2$) then we can find the complementary inverse temperature. As a simple example, suppose for $A_1$ we set the DW2X rescaling parameter $r = 0$ (or $\beta_T = 0$ for the STA), we would reasonably expect to recover $\beta = 0$, thereby the gap would be precisely $\beta_2$. Alternatively, we can estimate $\beta$ by one of the main text methods on only one of the two distributions, to complete the inference.

### 3.3 Estimation from multi-canonical methods

Two multi-canonical methods are explored experimentally here: the self-consistent multi-canonical (SCMC) approximation introduced in Section 3.2, and the linear regression multi-canonical (LRMC) method of Benedetti et al. [Benedetti et al. (2016)]. First, we discuss how multi-canonical methods may capture both local and global distribution features. We discuss limitations of multi-canonical methods, but also the fact that using the method in combination with MLPL (or some other single distribution estimator) can be used to efficiently indicate ergodicity breaking. We show in Section 3.5 some results demonstrating $\Delta\beta$ estimation in RAN1 problems. The results show patterns similar to those for the single distribution methods, but interpretation is difficult due to the interaction between rescaling and ergodicity breaking. In Section 3.4 we demonstrate the use of multi-canonical methods in isolating global and local effects. The choice of methods is not specific to the task in each subsection; we might leverage either method to achieve similar results in the respective sections.

Let us consider how two different annealer parameterizations may differ in distribution for the STA with the SCMC method (assuming qualitatively similar arguments for the DW2X, and for the LRMC method). Suppose two STAs differ in the terminal inverse temperature, in one case annealing to $A_1 = \beta_0$ and in the other case to $A_2 = (1 - \epsilon)\beta_0$, for relatively small $\epsilon$. With reference to Figure M1, we anticipate that both distributions are subject to a similar pattern of ergodicity breaking, but at the end of the anneal relax locally according to the different terminal inverse temperatures. The energy gap is a combination of energy gaps within each mode, and the energy gaps between modes. Restricting to replica-exchanges within the modes we may expect to see $\Delta\beta = \epsilon\beta_0$, but between modes of significantly differing energy, we would expect a much smaller value for $\Delta\beta$. If the energy gap between modes is large (as is the case schematically Figure M1) then the replica exchange probabilities between valleys will dominate the estimator, and we return an estimate close to zero. This is of course only one scenario, and depending on the relation between the rescaling and the ergodicity breaking we may see different patterns.

Since multi-canonical methods depend on both global and local features, we can infer ergodicity breaking by comparison with approximators that capture only local distribution features. We have two distributions and so can efficiently obtain MLPL estimates for each, as well as calculate $\Delta\beta$ by a multi-canonical estimate. Inconsistency of these estimates is an indicator of ergodicity breaking, but one which may be difficult to interpret independently of other knowledge about the distribution. This may be useful, but we caution that it cannot be relied upon to capture ergodicity breaking in general. Since it is self-consistent, and hence only sensitive to differences amongst observed modes, it will not capture ergodicity breaking related to the unseen modes (missing mass). This sensitivity to missing modes is a problem with any self-consistent estimation method, whether with a single distribution or multi-canonical. Another way to see ergodicity breaking, or perhaps simply bias in the estimators, would be to consider three pairs of distributions $(A_1, A_2, A_3)$, measuring $\Delta\beta$ between each. Of course, this should yield a consistent set of gaps if we have a Boltzmann distribution and unbiased estimators for the gap.

We would like to note a limitation of the energy gap matching criterion (S3). In order for the equation to be solved for some finite $\Delta\beta$ it is necessary that the range of the empirical distributions on energy overlap. Meaning, that the smallest energy of the hotter distribution is smaller than the largest energy on the colder distribution. In order to have low variance estimation we understand that the distributions ought to overlap strongly, otherwise the result is very sensitive to a small number of outliers in the energy distribution.

The LRMC method also has some shortcomings. Firstly, a linear regression method is employed. The objective being minimized, least squares, is not a particularly informative one and it is difficult to convert a

fitting error to useful information about the quality of the distributions. Secondly, a necessary feature of the method is that pairs of energy states are well occupied, which is a stronger requirement than in the SCMC method. Finally, the data points used in the fitting are noisy, and since the noise model will (at least for those low-occupancy energy levels) be non-Gaussian, a bias in estimation can be expected. Binning data so as to modify and mitigate for the errors, and to create compatible occupied levels, may itself introduce bias.

Aside from this we reiterate that use of multi-canonical methods have some disadvantages. Neither of the two methods have in our opinion been sufficiently and robustly tested, although the LRMC method has been successfully applied in a machine learning context. Both methods are consistent estimators, but bias and variance are poorly understood; perhaps a careful consideration of how to extract maximum information is required [Shirts and Chodera (2008)]. Also, the methods presented require collection of two sample sets (even if our interest is only in one parameterization) and potentially an assumption on $\Delta\beta$ as a function of the annealer parameterization. The assumption that $\beta$ is linear in the rescaling parameter is correct in the absence of ergodicity breaking; but based on analysis of Sections M4.5 and Section 3.5 requires some careful consideration.

### 3.4 Separation of global and local temperatures with the LRMC method

We evaluate the LRMC method in the context of the STA and the bidirectional associative memory model, described in Section 2. We note that our implementation of Benedetti et al. is simplified relative to the most recent version of their paper, so that we utilize data less efficiently [Benedetti et al. (2016)]. The model we evaluate has full bipartite connectivity, $128$ variables, and 3 well separated pairs of modes (modes for a given pair are related by a change of sign of all Ising spins). We use sample sets of size $10^4$, generated at two different terminal $\beta$ values ($A_1 : \beta_T = 4$ and $A_2 : \beta_T = 4x$, $x = 0.8$), in each case using a linear schedule in $\beta$ of $200$ sweeps.

To implement the LRMC method we first determine the energy that is most strongly represented in both sample sets. This *modal energy* $E_m$ is typically the ground state energy for this model-annealer combination. We then find all other relevant energy levels $E$: here we select energies that appeared at least $10$ times under both rescalings as relevant. This is because energy levels of low frequency are very noisy and we do not wish to introduce a noise model to complicate the story we present. If $\Omega_A(E)$ is the number of samples of energy $e$ under a rescaling $A$ then, assuming error bars are negligible, an estimate for $\beta$ is obtained by a least square fitting of the curve

$$\log\left(\frac{\Omega_{A_1}(E)}{\Omega_{A_1}(E_m)}\right) - \log\left(\frac{\Omega_{A_2}(E)}{\Omega_{A_2}(E_m)}\right) = \beta(1-x)(E-E_m)\ , \tag{S6}$$

Solving for $\beta$, by linear regression, gives the estimator for distribution $A_1$ according to the LRMC method.

In our presentation of the LRMC method we will also implement a variation, fitting independently data on 3 different subspaces as well as the full space. Each $E$ can be identified with one or more samples, and we can cluster these $E$ values according to which mode (memory) is at shortest Hamming distance (up to symmetry, there will be only 3 modes). We plot all the data points in Figure S1, but color them according to this classification. As can be seen, the data in its entirety is not well described by a linear fit, but after clustering we see that a linear fit on each mode seems appropriate. Within each mode we can obtain a local temperature describing the distribution on that mode, that is as expected close to $\beta_T$. Despite the use of $10^4$ samples, estimates are quite noisy due to the small sub-populations involved. Between the three curves there is a horizontal displacement: this reflects the fact that when we rescale the terminal $\beta$ by a factor $x = 0.8$ there is no significant redistribution between the modes. This is expected since

the ergodicity breaking happens early in the annealing procedure when the model is even further scaled down (approximately by $0.25$, if we trust the large $N$ behavior [Tanaka et al. (2000)]). Thus the two annealed distributions are macroscopically distributed between the modes in a similar manner. We can see how fitting all the data, as recommended by Benedetti et al., leads to a mixture of the global and local temperature [Benedetti et al. (2016)].

We have shown that multi-canonical methods, in combination with clustering, yields additional information. A combination of local and global distribution features is apparent in this example, which is easy to establish since we chose the model to induce clusters that would be well defined and easy to discover. However, some of this information could be extracted with single-distribution methods. In particular, we see that the local temperature estimates have strong variation about the expected value $\beta_T = 4$ in the example presented. If by contrast we cluster the points and apply the MLPL estimator to each mode independently we obtain estimates of much lower variance based on the same number of samples. In this sense, MLPL seems to use the local information more efficiently than the version of the LRMC method we have presented.

### 3.5 Rescaling dependence with the SCMC method

In this section we plot estimates to $\Delta\beta$ using the SCMC method. We study 100 RAN1 distributions under the DW2X sampling at various scales. In Figure S2 we compare two distributions that differ by $0.1$ (left) or $0.2$ (right) in the DW2X rescaling parameter. If we have equilibration at the terminal model, we anticipate a linear correspondence between the rescaling parameter and the inverse temperature, $\beta(r) \propto r$, and so we would expect a constant value. There is a clear departure. We determine larger gaps for the simpler models (smaller rescaling parameters, and smaller system size). The estimate for $\Delta\beta$ is also a non-linear function; the sum of $\Delta\beta$ for two successive pairs separated by $0.1$ in the rescaling parameter is not consistent with the estimate based on a single pair of models differing by $0.2$. Note that the absence of data points for larger systems and smaller $\beta$ is owing to the fact that the estimator is only usable when the energy distributions overlap, if the energy distribution support is disjoint $\Delta\beta$ is defined as infinite. The energy distributions are also quite well separated for larger system sizes (C12), so that these results might be considered relatively unreliable. In multi-canonical methods, as already noted, the rescaling should be chosen adaptively to allow reasonable overlap of the energy distribution.

The details of these curves are difficult to interpret, but under the approximation $\beta(r) \propto r$ we do however see trends qualitatively consistent with those discovered based on ML and MLPL estimation in Section 4.5. Rescaling to small values of $r$ we see larger inverse temperatures not far from the single qubit freeze-out prediction. For larger models we infer significantly smaller $\beta$ values, indeed much smaller even than those predicted by the maximum likelihood method in the case of large systems. As outlined in Section 3.3, it may be expected that when the samples are dynamically trapped by modes with strongly differing energies, the estimate will approach zero.

## 4 SAMPLING USING THE DW2X

### 4.1 Single qubit freeze-out in the DW2X

Figure M5(left) illustrates that local temperature, as measured by the MLPL method, is a non-linear function of the rescaling parameter. One can see that this temperature has only mild dependence on problem size (mild by comparison with the trend in ML). We illustrate this non-linearity again in Figure M7, where we find the local temperature of a trivial single qubit model $H(x) = x$ for the DW2X under different fields

(at various rescaling parameters $r$). This result can be compared with simulations of single qubit dynamics using the Redfield equation [Blum (2012); Weiss (1993)]. Using the best estimate of the annealing schedule of the DW2X with a $20\mu s$ anneal time (described in Section M4.3), and fitting a physical temperature parameter $T_{\rm phys} = 20.5{\rm mK}$ (in good agreement with the measured operational range), we are able to describe the non-linearity very accurately.

The origin of this non-linear dependency is the freeze-out of individual qubit dynamics at the end of the annealing process [Johnson et al. (2011); Amin (2015)]. The MLPL method estimates temperature by looking at the pattern of excitations on single qubits, in the context of the sample from which they were drawn. In the STA (and indeed in some simulations of quantum annealers - without physical dynamics) there is typically at least one update of all spins at the terminal temperature, so that within each sample spins are adjusted (locally) to the energy signal at the end of the anneal. This is the reason that the pattern of self-consistent spin excitations is consistent with $\beta_T$ in the STA (Figure M6), where the MLPL estimator indicates $\beta \approx \beta_T$ for any $\beta_T$. In physical quantum annealers, where the rate of transitions is controlled by the transverse field which changes throughout the anneal; the dynamics are fundamentally different. Since the transverse field becomes very small before the terminal energy scale is reached, the state of the qubit is controlled by the Hamiltonian operator at this intermediate point in the anneal.

Even though quantum dynamics as simulated by the Redfield equation are complex in the case of a single qubit, there is a very simple explanation for the shape of the effective temperature curve. Assuming that late in the anneal the physical temperature is negligible in the single qubit dynamics, the transition rate for single qubits is found to be determined exclusively by the ratio $\alpha(s) = \frac{E(s)}{\Delta(s)}$, where $E(s)$, $\Delta(s)$ are the envelope functions described in Section M4.3. We determine from the Redfield simulation with rescaling parameter $r = 1$ the single qubit dynamics freeze-out at $s^* = 0.65$ (or 13 $\mu s$ during an anneal of 20 $\mu s$). This means that the single qubit distribution reflects a locally equilibrated distribution at $\alpha^* = \alpha(s^*)$. The effective inverse temperature describing this point will be proportional to the energy scale $E(s^*)$. Now if we submit the problem under a new rescaling parameter $r < 1$, freeze-out will happen at a later time $s(r)$ where $\alpha(s(r)) = \alpha^*$ and the effective inverse temperature will be proportional to $rE(s(r))$.

Figure M7 shows good agreement between this single qubit freeze-out effective temperature and the Redfield simulation. Thus in the case of a single qubit the non-linear dependence of effective temperature on the rescaling parameter is determined by the annealing schedule.

## 4.2 Implications of the single qubit result for other ensembles

We can extend the concept of single qubit freeze out so that it can describe patterns of local temperature via MLPL for general multi-qubit problems. We will appeal to a classical argument that appears to explain some features of the non-linearity, and differences amongst problem classes and system sizes. As described in Section 5, the MLPL estimator is determined by examining the effective fields on individual qubits in sampled states

$$\zeta_i = h_i + \sum_j (J_{ij} + J_{ji}) x_j \ . \tag{S7}$$

At the single-qubit freeze-out point the dynamics of individual qubits will slow down, and the state will evolve according to a local field operator analogous to (S7). If the neighbors of a spin take prescribed classical states, then the spin will evolve late in the anneal equivalently to a single qubit in a field. The MLPL estimator accumulates a signal from the pattern of excitations on all sites and in every sample, and smaller (but non-zero) values of $|\zeta_i|$ contribute most significantly to this signal. For a given problem there is a distribution of $|\zeta_i|$ so a single curve such as Figure M7 is insufficient. However, we may anticipate the

result as a weighted average of such curves that varies only slightly amongst problems of a given class. Concavity of MLPL curves is therefore to be expected, except where many $|\zeta_i|$ are small (but non-zero) and we are in the near-linear regime of the curve (Figure M7).

From our samples, we can approximate separately a value of $\zeta_i$ for every variable, in every sample, late in the anneal. In the RAN1 problems ($h_i = 0$, $J_{ij} = \pm 1$) only a limited set of integer values for $\zeta_i$ are possible. For $|\zeta_i| = 1$, the qubit had a freeze-out characterized by the inverse temperature for $r = 1$ in Figure M7. However, the majority of non-zero local fields will be larger ($|\zeta_i| \geq 2$), and these freeze-out even earlier (at smaller $\beta$). The MLPL estimate will merge these values, so that we find something intermediate. A simple explanation for the trend of decreasing $\beta$ with system size in Figure M6(left) would therefore be that we see fewer instances of $|\zeta_i| = 1$ relative to $|\zeta_i| \geq 2$; this is indeed the case.

In the AC3 problem couplings $|J_{ij}|$ take values $1/3$ and $1$ and effective fields will often be as small as $|\zeta_i| = 1/3$. These qubits freeze-out significantly later than the RAN1 counterparts, and so are characterized by larger MLPL estimates of $\beta$. This is consistent with the observed pattern in Figure S3(left) that AC3 MLPL $\beta$ estimates are larger than those for RAN1, are weakly dependent on system size and have approximately linear scaling with $r$. This is discussed further in Section 8, where AC3 results are presented.

The MLPL estimator ($\hat{\beta}_{MLPL}$) merges the estimates coming from sizes of large $|\zeta_i|$ with those of small $|\zeta_i|$. However, we can build locally-consistent estimators to tease apart contributions. For example, it is valid to define an estimator (by choice of the Kernel) to separately consider excitations over even connectivity sites ($\hat{\beta}_{even}$) where the smallest non-zero $|\zeta_i|$ is 2, and odd connectivity sites ($\hat{\beta}_{odd}$) where the smallest non-zero $|\zeta_i|$ is 1. These estimators agree up to statistical error in the STA, or drawing perfect samples, but in the DW2X $\hat{\beta}_{even} < \hat{\beta}_{MLPL} < \hat{\beta}_{odd}$. We have found similar trends in studying ensembles with special connectivity distributions [King et al. (2016)]. This is precisely the kind of local deviation that can be cleaned up by post-processing.

King et al. have previously noted that the distribution of effective fields, and by extension the degree distribution in RAN1 problems, can have a significant impact on the late anneal quantum dynamics [King et al. (2016)]. Our explanation is purely classical, but seems to explain the trends with respect to problem classes and problem sizes quite well. However, at this stage we cannot rule out a role for multi-qubit freeze-out quantum phenomena in MLPL estimation.

### 4.3 DW2X sampling

Proceeding (infinitely) slowly, so that equilibration occurs at the terminal model, we would be guaranteed to sample a diagonalized state described by a Boltzmann distribution Eq. (M2) coincident with the classical Hamiltonian Eq. (M1). Equating the prefactors for the two unitless Hamiltonians we have $\beta_0 = hE_{max}/(2k_BT) = 11.3$, which is the terminal inverse temperature – the expected overall scaling of the Hamiltonian. In Section 4.1 it was discussed why we do not equilibrate at this inverse temperature, and why the inverse temperature we do find is not necessarily a linear function of the rescaling parameter $r$.

A number of noise sources affect the components of the processor, aside from temperature fluctuations. These have been increasingly mitigated with each generation of D-Wave processors and by calibration efforts, but remain significant in the processor used [Denil and de Freitas (2011); King et al. (2015a); Yoshihara et al. (2006); Harris et al. (2008)]. A simple model for the combined effect of error sources is one of independent zero-mean Gaussian distributed offsets on each programmed field and coupling; fitting this model to data for simple Hamiltonians estimates for the variance of $0.05^2$ for fields, and $0.035^2$ for couplings have been established in some systems (relative to a programming range of $[-1, 1]$ for J

and $[-2, 2]$ for h) [King et al. (2016); Venturelli et al. (2015); Dumoulin et al. (2015)]. Such a model can provide intuition for the scale of noise, and the precision available to programmers; but does not account for time dependence in the noise sources, some systematic errors, and cross talk.

### 4.4 Impact of spin reversals on the DW2X distributions

A spin reversal transformation of the Hamiltonian is defined by a random vector $\eta \in \{-1, 1\}^N$. Given such a vector we can define a new Hamiltonian

$$H_\eta(x) = \sum_{ij} J_{ij}\eta_i\eta_j x_i x_j + \sum_i \eta_i h_i x_i \tag{S8}$$

Boltzmann samples drawn according to this distribution $\mathcal{S}_\eta = \{x\}$, can be transformed in Boltzmann samples on the original distribution, by componentwise multiplication of every sample by $\eta$. This is due to a symmetry. Any reasonable heuristic will respect such a transformation, thus the rule for Boltzmann samplers applies also to good heuristics in principle.

Although the DW2X is designed to obey this symmetry, it is weakly violated due to noise sources. Fortunately, spin-reversal transformations can be used to mitigate for the noise sources that cause this symmetry breaking. To do this, we can draw each sample according to a different spin-reversed Hamiltonian (S8), transforming by a random vector $\eta$, and reversing this transformation to obtain a sample in our original space. In this way, the random impact of noise on each representation is *averaged out* at the distribution level.

For purposes of our study, using many spin-reversal symmetries is also valuable in reducing autocorrelation of the samples. We find that whereas samples drawn sequentially for a fixed programming ($\eta = \mathbf{1}$) have some measurable autocorrelation that decays according to a $1/f$ spectrum [Lanting et al. (2009)]. The autocorrelation on statistics derived from samples that each differ by spin-reversal transformations is difficult to detect.

Unfortunately, it is currently very impractical to use a separate spin-reversal transformation for every sample, since each Hamiltonian submission must be programmed, requiring some time. It is more time efficient to draw samples in batches. In Figure M2 we show how the distributions err from the Boltzmann distribution as a function of the number of spin-reversals used in generating the sample set (total sample set size is normalized, so this uncertainty is removed). There is clearly a very large improvement in moving from sets constructed from one spin-reversal to sets constructed of 10 or more, but beyond this the returns are diminishing. For this reason we used for the bulk of our studies the more efficient format of 10 spin-reversals by 1,000 samples.

### 4.5 Effects of embedding on temperature estimation

When we sample from an embedded problem we obtain a distribution on the qubit states, not on the “logical states” of the original problem. We can create a distribution on the “logical space” problem by projecting samples into that space. The embedding we use utilizes chains to enforce identity relations amongst qubits, so that when chains are intact we are in a subspace that has a one-to-one mapping in energy back to the logical space problem. Samples in this subspace can be converted directly into samples on the logical problem, and if the distribution is Boltzmann on the embedded space, it will be Boltzmann on this subspace (thereby the logical problem), and with the same parameter $\beta$.

Samples that violate these chains may be numerous, and can be brought into the chain-intact subspace by error correction methods (these can be thought of as post-processing in the embedded space). Most naive amongst these methods is chain voting (assigning all values in a chain to the value most represented in the chain). This is the only form of projection evaluated in this paper – more sophisticated projecting methods would involve a more careful study of the difference in the energy landscapes and perhaps a consideration of quantum chain dynamics.

We consider a single instance of a $40$ variable NAE3SAT problem. This is an exemplar for the behaviour we see in this problem and in some other related problems such as the BAM model (which we have also tried embedding). For this instance the process of embedding transforms the Hamiltonian (S2) on $40$ variables into a Hamiltonian on $308$ qubits[2]. The energy penalty per embedding violation is chosen to be $1.80$ (in the unscaled units of (S2)), reflecting a trade-off amongst various quantum annealing features (particularly precision). In other words, an embedding violating excitation is roughly twice as expensive as a clause violating excitation. When drawing $10^4$ samples we see approximately $12.5\%$ of samples are chain-intact, so that the majority of samples contain at least one embedding violation.

In Figure S4(left) we show the energy distribution of the samples in the $308$ dimensional qubit space, evaluated according to the embedded Hamiltonian, and three Boltzmann distribution. We use parallel tempering to determine the mean energy and energy histogram for each of the Boltzmann distributions. In Figure S4(right) we consider the energy distribution in the $40$ dimensional logical space of the original problem for the subset of samples that were chain-intact, and for all samples (after these are chain-voted into the lower dimensional space), as well as the same three Boltzmann distributions. The Boltzmann distributions were chosen by the maximum likelihood criteria with respect to the three hardware distributions that are plotted, and each distributions seem to be in qualitative agreement with some Boltzmann distribution – but not the same one. The error bars associated to the chain-intact distribution reflecting only the fact that we have fewer chain-intact samples from which to estimate. We use dynamic programming to determine the mean energy and energy histogram for each of the Boltzmann distributions. There is reasonable agreement of all three DW2X derived distributions with the energy spectrum of some Boltzmann distribution. However, we caution that this does not guarantee that the MSE on correlations, or some other statistic weakly dependent on the energy spectrum, will also be Boltzmann. We did not thoroughly test in this regard.

We can see that in the embedded problem the value of $\beta$ that best describes the mean energy is relatively large. By contrast the estimate over the subspace where chains are intact is slightly smaller. Including chain-voted samples alongside the chain-intact samples decreases the $\beta$ estimate on the subspace (we introduce relatively more high energy states). If the distribution is Boltzmann in the embedded space, then the same distribution ($\beta$) describes the chain-intact subspace, and therefore the logical problem on $40$ variables. In this example (and in others not presented) we find this not to be the case: $\beta$ measured on the embedded space would predict too large a mean energy if applied to the logical problem.

Since the objective may be to sample at larger inverse temperature in the logical space, we must consider whether inclusion of the chain-broken samples (whether by chain-voting, or some other mechanism) is valuable. If we restrict to the chain-intact system it seems we have a Boltzmann distribution at significantly lower temperature; including chain-broken states we have more samples, but we also move to smaller $\beta$ where it is easier to sample by alternative means. Note that the situation in sampling is much more

[2] We use the standard embedding function provided by the application interface for the DW2X, based on the standard heuristic [Cai et al. (2014)]. This embeds onto a C8 subgrid of the DW2X graph for the problem presented.

complicated than the situation in optimization - in optimization we do not have to worry about the distribution over the lowest energy states, merely the extreme value. In this sense projecting samples (e.g., by chain voting) does no harm, whereas this is not true in sampling.

## 5 MAXIMUM LOG-PSEUDO-LIKELIHOOD

Maximum log-pseudo-likelihood (MLPL) is an attempt to replace the maximum likelihood estimator by a tractable one [Besag (1975); Bhattacharya and Mukherjee (2015); Aurell and Ekeberg (2012)]. This is a common heuristic in parameter estimation, although it is more commonly applied for larger parameter sets, as a cheap alternative to iterative minimization procedures.

The pseudolikelihood estimate might be achieved by the following substitution for $P_\beta(x)$ in (M3)

$$P_\beta^{PL}(x) = \prod_i B_\beta(x_i | x \setminus x_i) \tag{S9}$$

and minimizing with respect to $\beta$. This method can be justified by its results, and rederived in other ways, but is sometimes difficult to interpret – notably (S9) is not a probability.

Maximum likelihood estimation requires the NP-hard to calculate quantity of mean energy. Pseudo likelihood allows us to bypass this hard inference task. One way to think about the additional power of pseudo-likelihood is that it uses additional information from every sample, not just the essential statistic, energy - which is all that is used in a maximum likelihood estimate [Aurell and Ekeberg (2012); Montanari (2015)].

As discussed in Section 3.1 we can derive the same estimate for $\beta$ from the energy matching criterion (M4) averaging over all possible single bit-flip resamplings (M9). This provides a clear interpretation for the method, and presents natural generalizations.

## 6 EXTENSIONS OF THE SELF-CONSISTENT APPROXIMATION

The maximum log-pseudo-likelihood estimator is determined by the energy matching criterion under the self-consistent approximation (M7), with single bit resampling (M9). Our argument throughout this paper has been that all choices for $W_\beta$ will likely lead to quantitatively similar *local* estimates of $\beta$, as they redistribute samples only locally and preserve macroscopic biases. In this section we demonstrate that the situation is slightly more blurred. One implementation of (M7) in this section is to take $W$ to be a sequence of $m$ sweeps of blocked Gibbs, and to solve the energy matching criterion under this sequence of increasingly powerful approximations. As $m$ goes to infinity we would recover $B_\beta$ perfectly, and so obtain the global estimate to inverse temperature, for small $m$ the approximation is increasingly local as $m$ decreases. MLPL is even more local than single-sweep, and so produces an even higher estimate to $\beta$.

In Figure S5 we demonstrate the inverse temperature estimates obtained as a function of the different self-consistency criteria ($m$). Results are for sampling of 100 random $40$ variable NAE3SAT problems using the DW2X; the samples are obtained by embedding the Hamiltonian and “chain-voting” the samples into the $N = 40$ dimensional logical space (see Section 4.5 to understand chain voting). In this way each of the $10^4$ anneals yields a sample.

In Figure S5(left) we show the energy matching value $\mathrm{EM}(\beta)$ (M4) for 100 different problem instances under $m = 1$ sweep of blocked Gibbs sampling approximation. Setting $\mathrm{EM}(\beta) = 0$ we obtain the

Maximum Likelihood estimate. In the Figure S5(right) we demonstrate how, as we increase the amount of post-processing $m$, the median estimate of $\beta$ evolves downwards, towards the maximum likelihood estimate. Errors in Figure S5(right) represent uncertainty associated to the blocked Gibbs procedure itself, which was repeated many times per initial condition $P_A$. In the distribution over 100 instances there is significantly more variation.

We can see that self-consistent approximations can be improved and yield values closer to the maximum likelihood estimate (and further from the MLPL estimate) by increasing the power of the kernel $W$ used in the post-processing method. This problem is however a very small one, of only $40$ variables, and effects are less pronounced in larger hard problems.

## 7 KLD ESTIMATION WITH MIXTURE MODELS ON SUBSPACES

The KL-divergence (M3) can be expressed as an entropy, a mean energy scaled by $\beta$, and a log partition term

$$D_{KL}[P_A, B_\beta] = -\left[-\sum_x P_A(x)\log P_A(x)\right] + \beta \sum_x P_A(x)H(x) + \log(Z(\beta)) \ . \tag{S10}$$

We can determine a value of $\beta$ minimizing this quantity through the energy matching criterion, but to understand quality we should evaluate this objective. An obvious problem is the evaluation of $\log(Z)$, which is NP-hard. Nevertheless, methods such as annealed importance sampling or parallel tempering can be effectively employed for the problem types we have presented [Geyer and Thompson (1992); Neal (2001)].

Unfortunately evaluation of the entropy term from a set of samples is also problematic. Entropy is a non-linear function of $P_A$, and when estimated by plug-in type approaches (M6) is subject to strong bias [Paninski (2003); Grassberger (2003)]. The plug-in estimator based upon (M6) yields a consistent estimator, but it is only when $\log$ of the number of samples is greater than the entropy that we may accurately estimate the entropy term. Boltzmann distributions have entropy that grows linearly with the dimensionality. Thus, it seems that unless we make some strong assumption on the distribution $P_A$ then we cannot capture the entropy term.

An example where we have such additional information is a post-processed distribution (M11), which we have also argued in Section 4.7 of this paper provides more meaningful information on the practical usefulness of the samples obtained from annealing. If we evaluate the KL-divergence for this distribution we can exploit knowledge of the analytical form for $W_\beta$ to improve estimation, both the bias and variance of the crude estimator. The use of this analytical form can be interpreted as Rao-Blackwellization, with respect to the KLD of the post-processed distribution. It can also be shown that the KL-divergence of the post-processed distribution provides a lower bound on the KL-divergence for the unprocessed distribution, thus this quantity provides useful information on the unprocessed heuristic distribution.

We can develop this idea for blocked Gibbs post-processing of a bipartite Ising model. In a bipartite model, there are two sets of variables $\mathcal{S}$ and $\mathcal{T}$, that are each conditionally independent (disconnected in the graphical model). If we first conditionally sample $\mathcal{S}$ according to the Boltzmann distribution, and then $\mathcal{T}$, this is one sweep of blocked Gibbs sampling. The new set of samples are described by a post-processed distribution (M11) with the kernel

$$W(x|x') = B_\beta(x_S|x_T)B_\beta(x_S|x_T) \ . \tag{S11}$$

Evaluating the KL-divergence for $P_{A,\beta}$ under this kernel, we are able to simplify the expression to

$$D_{KL}[P_{A,\beta}, B_\beta] = E\left[\log\left(\frac{P_{A,\beta}(x_S)}{B_\beta(x_S)}\right)\right] \; , \tag{S12}$$

where $E[\cdot]$ is an expectation with respect to $P_{A,\beta}(x_S)$. If we then take the plug-in estimator to the original annealing distribution $P_A$ (M6), we are able to approximate $P_{A,\beta}$ as

$$\hat{P}_{A,\beta}(x_S) = \sum_{x_T} \hat{P}_A(x_T) \prod_{i \in S} \frac{\exp(\beta\zeta_i(x_T)x_i)}{2\cosh(\beta\zeta_i(x_T))} \tag{S13}$$

where $\zeta(x) = (J + J^T)x + h$; $\zeta_i(x)$ is a function only of $x_T$ for $i \in S$ due to the bipartite structure. The new expression (S12) cannot be exactly evaluated in polynomial time, but perfect sampling from $P_{A,\beta}$ is possible. We can thus obtain an accurate estimate by evaluating the expectation by Monte Carlo sampling. Some tricks outlined in [Jaakkola and Jordan (1998)], who evaluate a similar functional form in the context of a different method, can be brought to bear in reducing this variance.

Two things have changed relative to estimating KL-divergence with a plug-in estimator. Firstly, we are evaluating the KL-divergence for distributions on a subspace $S$ that is half as large as the original space $S \cup T$, secondly the distribution $P_{A,\beta}$ is not determined by a histogram on samples, but as a mixture of product distributions. Each of these features allows us to exponentially reduce (exponential in the dimensionality of the system, $N$) the number of samples required to accurately estimate KL-divergence.

Using the estimator (S12) we show results in Figure M14 for the KL-divergence for a single typical instance from both RAN1 and AC3 problem classes at C4 scale (127 variable); there is strong variation between instances at this scale, but the two patterns are exemplars chosen to be typical in the maximum likelihood estimate for $\beta$. Solid lines indicate the estimator, and dashed lines indicate the jack-knife bias corrected estimate [Efron (1982)], the fact that the bias is appreciable even with $10^4$ samples is an indication that we are approaching the limit of usefulness of this estimator. Indeed, the bias for the $40$ sweep STA is so large as to render the estimate of entropy ineffective; the case of $400$ sweeps is marginal, whereas for the $4000$ sweep STA, and the DW2X, the estimates are accurate everywhere.

With $10^4$ samples we would, in the absence of the post-processing trick, be limited to estimating KL-divergence for distributions of entropy $\lesssim \log(10^4) = 9.4$; however, in this case we accurately measure entropy even as $\beta \to 0$ (where entropy is $128\log(2)$). The KL-divergence objective indicates strong performance at low temperature for the DW2X, a reflection of the ability to reach consistently low energy scales [King et al. (2015b)]. If we instead used the MSE objective (M5) across this range of $\beta$ we find that the STA performance is improved relative to the DW2X.

Unfortunately, the use of this estimator is still fundamentally limited by the curse of dimensionality. To understand the limitations of this estimator we can consider first the best case scenario for performance, when the parameters $\zeta(x_T)$ happen to be optimal (minimizing the KL-divergence). The KL-divergence would then match that for a mixture of mean-field approximations [Jaakkola and Jordan (1998)]. In this context we can assert that the KL-divergence for a single mixture component (derived from a single sample) can be no better than the mean-field approximation. The KL-divergence of a mean-field approximation can be quite poor, except in the approximation of a single mode and the KL-divergence between a mean-field approximation and many interesting Boltzmann distributions can be expected to grow linearly with the dimensionality. Also shown in [Jaakkola and Jordan (1998)], is the fact that the KL-divergence decreases

at most logarithmically in the number of mixture components (number of samples). In this scenario, we may still require a number of samples that is exponential in the dimensionality if we are estimating for a distribution that is close to a Boltzmann distribution.

This can be restated more informally. We know that a single sample processed by one sweep of blocked Gibbs may spread quite representatively over one mode of the distribution, and so capture local energy and entropy. However, if there are a large number of modes (including local minima which trap dynamics), then we need to see them all many times to begin estimating the inter-mode entropy term (also called complexity [Mezard and Montanari (2009)], capturing the distribution over modes) correctly. In the case of RAN1 we find that quite quickly, beyond scale C4, the estimator can become strongly biased in a qualitatively similar manner to the plug-in estimator, particularly at intermediate temperatures; for this reason in the main text we have chosen MSE as our objective of choice.

# 8 ESTIMATING $\beta$ IN AC3 PROBLEMS

In Figure S3 we show results from the DW2X for AC3 problems. In contrast to the RAN1 results in Section 4.5, here the MLPL method of estimating local $\beta$ is much closer to the linear. The maximum likelihood estimator, however, still reflects the global distribution distortions due to ergodicity breaking. It is worth noting that both estimators show the DW2X to be sampling from colder temperatures than in the RAN1 case. We understand that higher precision problems may be expected to have MLPL estimates that scale linearly with the DW2X rescaling parameter, as discussed in Section 4.1. Simulated thermal annealing results show the same qualtitive features as Figure M6, and are not presented.

# 9 SUPPLEMENTARY TABLES AND FIGURES

## 9.1 Figures

## REFERENCES

Hen I, Job J, Albash T, Rønnow TF, Troyer M, Lidar DA. Probing for quantum speedup in spin-glass problems with planted solutions. *Phys. Rev. A* **92** (2015) 042325.

King AD, Lanting T, Harris R. Performance of a quantum annealer on range-limited constraint satisfaction problems (2015a). ArXiv:1502.02098.

King AD, Hoskinson E, Lanting T, Andriyash E, Amin MH. Degeneracy, degree, and heavy tails in quantum annealing. *Phys. Rev. A* **93** (2016) 052320. doi:10.1103/PhysRevA.93.052320.

Zhu Z, Ochoa AJ, Schnabel S, Hamze F, Katzgraber H. Best-case performance of quantum annealers on native spin-glass benchmarks: How chaos can affect success probabilities. *Phys. Rev. A* **93** (2016) 012317.

Katzgraber HG, Hamze F, Andrist RS. Glassy chimeras could be blind to quantum speedup: Designing better benchmarks for quantum annealing machines. *Phys. Rev. X* **4** (2014) 021008.

Mezard M, Montanari A. *Information, Physics, and Computation* (New York, NY, USA: Oxford University Press, Inc.) (2009).

Douglass A, King AD, Raymond J. *Theory and Applications of Satisfiability Testing – SAT 2015: 18th International Conference, Austin, TX, USA, September 24-27, 2015, Proceedings* (Cham: Springer International Publishing), chap. Constructing SAT Filters with a Quantum Annealer (2015), 104–120.

Janson A, Luczak T, Rucinski A. *Random Graphs* (New York, NY, USA: John Wiley & sons) (2000).

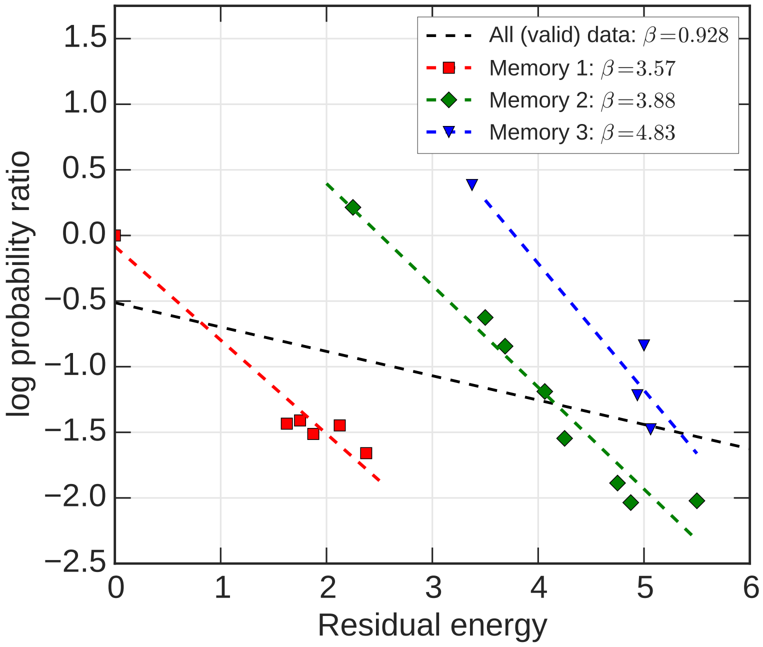


**Figure S1.** Log empirical frequency ratios are shown versus the residual energy (energy of the state minus energy of the ground state), the gradient characterizes a temperature. Energies are classified into modes by color, according to their nearest memory (Hamming distance). Each mode is well fitted by a single curve, which describes the local temperature and is in rough agreement with the target temperature, $\beta_T = 4$, as would be expected in the STA. Between modes data are displaced horizontally. The three upper most points describe local ground states and do not show a decreasing trend – indicating that the rescaling by a factor $x = 0.8$ has little effect on the relative probabilities of local ground states relative to the global ground state. A linear fit to all the data gives a temperature that mixes this global distribution feature, with the contribution of the local estimates. A naive linear fit is made in each case, excluding analysis of errors on data points (errors on points grow moving rightward and downward, as state frequencies decrease).

Landau DP, Binder K. *A Guide to Monte Carlo Simulations in Statistical Physics* (Cambridge, UK: Cambridge University Press), 2nd edn. (2005).

Cai J, Macready B, Roy A. A practical heuristic for finding graph minors (2014). ArXiv:1406.2741.

Bart K. Bidirectional associative memories. *IEEE transactions on systems, man, and cybernetics* **18** (1988) 49–60.

Tanaka T, Kakiya S, Kabashima Y. Capacity analysis of bidirectional associative memory. *Proc. Seventh Int. Conf. Neural Information Processing, Taejon, Korea* (Citeseer) (2000), vol. 2, 779–784.

Benedetti M, Realpe-Gómez J, Biswas R, Perdomo-Ortiz A. Estimation of effective temperatures in quantum annealers for sampling applications: A case study with possible applications in deep learning. *Phys. Rev. A* **94** (2016) 022308. doi:10.1103/PhysRevA.94.022308.

Hukushima K, Nemoto K. Exchange Monte Carlo method and application to spin glass simulations. *Journal of the Physical Society of Japan* **65** (1996) 1604–1608.

Shirts MR, Chodera JD. Statistically optimal analysis of samples from multiple equilibrium states. *The Journal of Chemical Physics* **129** (2008) 124105.

Blum K. *Density matrix theory and applications; 3rd ed.*. Springer Series on Atomic Optical and Plasma Physics (Berlin: Springer) (2012).

Weiss U. *Quantum dissipative systems* (Singapore: World Scientific) (1993).

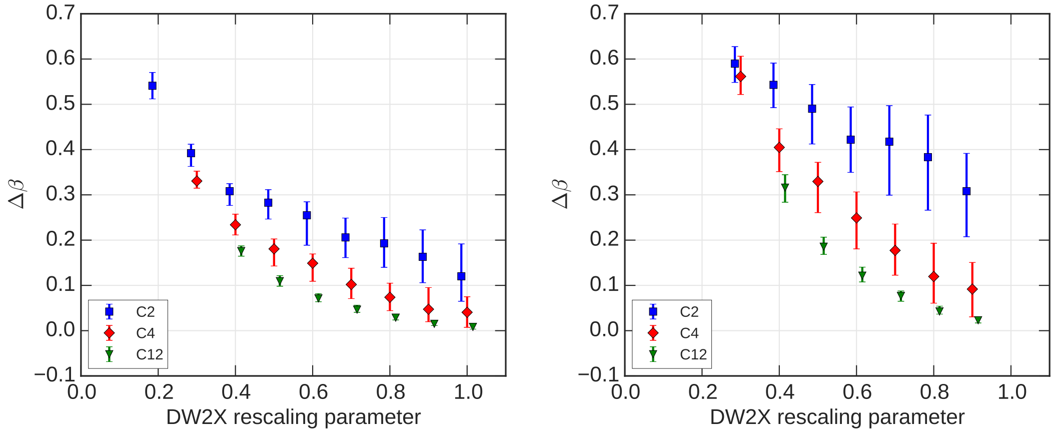


**Figure S2.** $\Delta\beta$ estimates in RAN1 models using the multi-canonical approach. Where points are absent the estimate is infinite due to non-overlap of the energy distributions at the different parameter settings. Error bars represent median and quartiles with respect to 100 instances studied. (left) 9 pairs of annealing distributions differing in the DW2X rescaling parameter $(r, r-0.1)$ were used, $r = 0.2, \ldots, 1$. (right) 8 pairs of annealing distributions differing in the DW2X rescaling parameter $(r, r-0.2)$, $r = 0.3, \ldots, 1$.

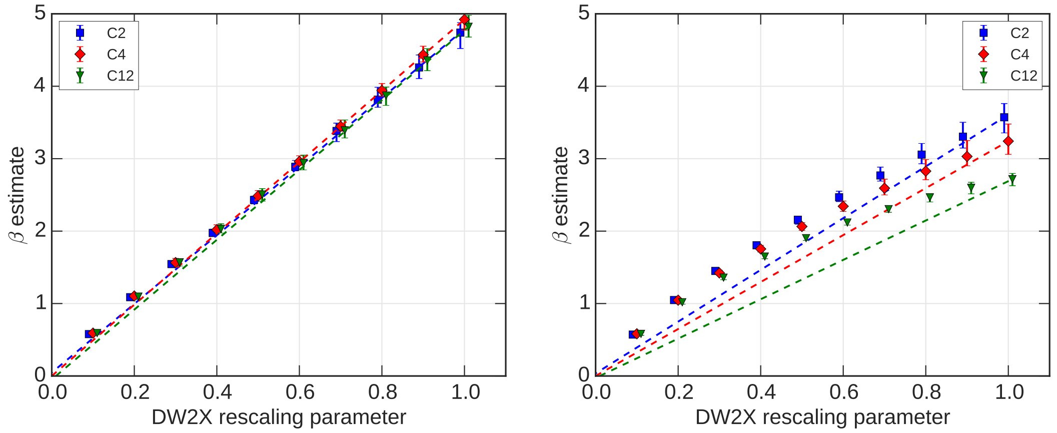


**Figure S3.** Bars represent quartiles over 100 random instances of AC3 at each scale. (left) Temperature estimates by the MLPL method. (right) Temperature estimates by maximum likelihood.

Johnson MW, Amin MHS, Gildert S, Lanting T, Hamze F, Dickson N, et al. Quantum annealing with manufactured spins. *Nature* **473** (2011) 194–198.

Amin MH. Searching for quantum speedup in quasistatic quantum annealers. *Phys. Rev. A* **92** (2015) 052323. doi:10.1103/PhysRevA.92.052323.

Denil M, de Freitas N. Toward the implementation of a quantum RBM. *NIPS 2011 Deep Learning and Unsupervised Feature Learning Workshop* (Cambridge,MA: MIT Press) (2011), vol. 5.

Yoshihara F, Harrabi K, Niskanen AO, Nakamura Y, Tsai JS. Decoherence of flux qubits due to $1/f$ flux noise. *Phys. Rev. Lett.* **97** (2006) 167001.

Harris R, Johnson MW, Han S, Berkley AJ, Johansson J, Bunyk P, et al. Probing noise in flux qubits via macroscopic resonant tunneling. *Phys. Rev. Lett.* **101** (2008) 117003.

Venturelli D, Mandrà S, Knysh S, O'Gorman B, Biswas R, Smelyanskiy V. Quantum optimization of fully connected spin glasses. *Phys. Rev. X* **5** (2015) 031040.

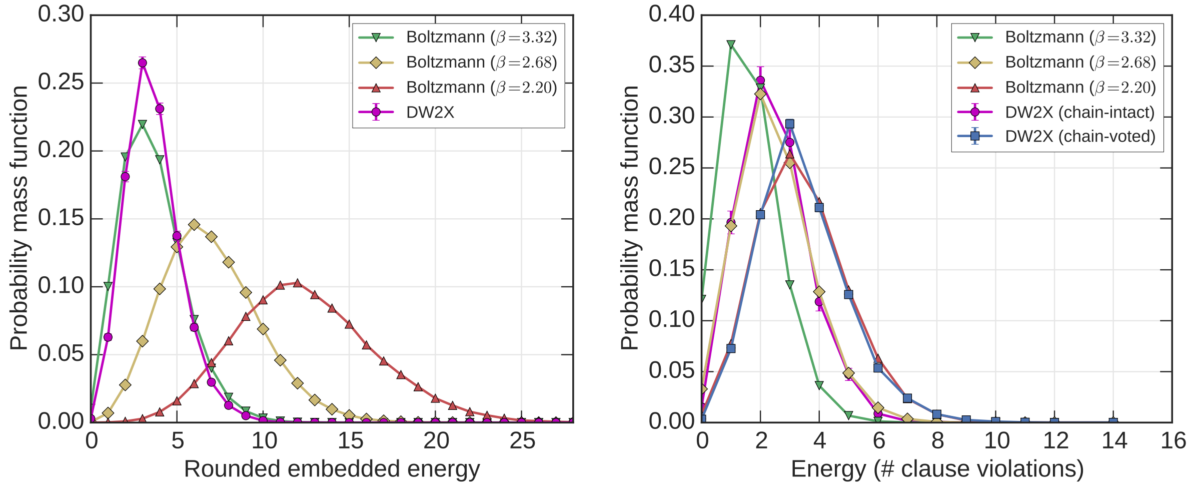


**Figure S4.** The Boltzmann distribution for the embedded problem (left) differs from the Boltzmann distribution in the logical space (right). The characteristic temperature is also a function of the utilization of samples. To obtain a set of samples in the variable space we either take only those chain-intact samples (discarding all other cases), or we take all samples chain-voted (projecting the chain-broken cases onto chain-intact ones). Whether we include chain-broken samples or not affects the temperature we estimate, as does whether we evaluate in the space of the original problem, or the embedded space.

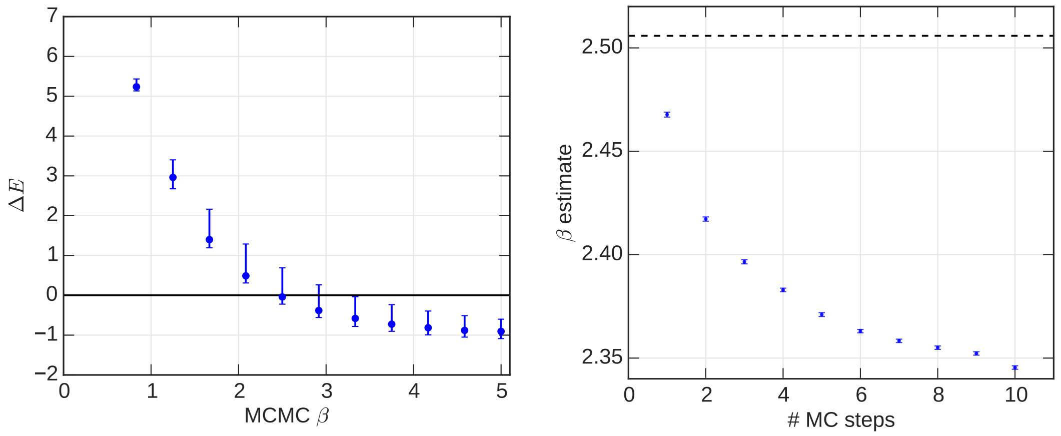


**Figure S5.** Median and quartiles over a set of 100 NAE3SAT problems (40 variables, clause-to-variable ratio of 1.8). (left) $\mathrm{EM}(\beta)$, the deviation from the energy matching criterion (M4) is shown as a function of $\beta$ used in our one sweep of blocked Gibbs approximation to $B_\beta(x)$. When $\Delta E = 0$ we have an approximation to the maximum likelihood estimator. (right) Estimation of $\beta$ using blocked Gibbs self-consistency as a function of increasing number of sweeps; as we move to larger number of sweeps we move towards the maximum likelihood estimate of $\beta$, and further from the MLPL estimate (shown as the dashed line).

Dumoulin V, Goodfellow I, Courville A, Bengio Y. On the challenges of physical implementations of RBMs. *Proceedings of the 28th AAAI Conference on Artificial Intelligence.* (2015). ArXiv:1312.5258v2.

Lanting T, Berkley AJ, Bumble B, Bunyk P, Fung A, Johansson J, et al. Geometrical dependence of the low-frequency noise in superconducting flux qubits. *Phys. Rev. B* **79** (2009) 060509. doi:10.1103/PhysRevB.79.060509.

Besag J. Statistical analysis of non-lattice data. *Journal of the Royal Statistical Society. Series D (The Statistician)* **24** (1975) pp. 179–195.

Bhattacharya BB, Mukherjee S. Inference in Ising models (2015). ArXiv:1507.07055.

Aurell E, Ekeberg M. Inverse Ising inference using all the data. *Phys. Rev. Lett.* **108** (2012) 090201.

Montanari A. Computational implications of reducing data to sufficient statistics. *Electron. J. Statist.* **9** (2015) 2370–2390.

Geyer CJ, Thompson EA. Constrained Monte Carlo maximum likelihood for dependent data. *Journal of the Royal Statistical Society. Series B (Methodological)* **54** (1992) 657–699.

Neal RM. Annealed importance sampling. *Statistics and Computing* **11** (2001) 125–139.

Paninski L. Estimation of entropy and mutual information. *Neural Comput.* **15** (2003) 1191–1253.

Grassberger P. Entropy estimates from insufficient samplings (2003). Arxiv:physics/0307138.

Jaakkola TS, Jordan MI. *Learning in Graphical Models* (Dordrecht: Springer Netherlands), chap. Improving the Mean Field Approximation Via the Use of Mixture Distributions (1998), 163–173. doi:10.1007/978-94-011-5014-9_6.

Efron B. *The Jackknife, the bootstrap and other resampling plans*. CBMS-NSF Reg. Conf. Ser. Appl. Math. (Philadelphia, PA: SIAM) (1982). Lectures given at Bowling Green State Univ., June 1980.

King J, Yarkoni S, Nevisi MM, Hilton JP, McGeoch CC. Benchmarking a quantum annealing processor with the time-to-target metric (2015b). ArXiv:1508.05087.
